# Supplementary material for: Flow regimes of Rayleigh-B\'enard convection in a vertical magnetic field
Source: arXiv:2002.07414 ancillary file (2020-02-18)
Supplement: Supplementary file 1 [file Supplement_data_table.pdf]

Supplementary material for the article *Flow regimes of Rayleigh-Bénard convection in a vertical magnetic field* by Till Zürner, Felix Schindler, Tobias Vogt, Sven Eckert and Jörg Schumacher.

This document contains selected quantities over the $(Ra, Ha)$ parameter range presented in the main article. Uncertainties of the quantities are given as standard deviation. The *Figure* column gives a reference to which measurements are specifically shown in a figure of the main article. More details on the definition of the listed quantities can be found in the main article.

## Measurements without magnetic field

The following measurements at $Ha = 0$ and are in the *LSC: Oscillations* regime. The uncertainties of $Pr$ and $Pm$ are, at most, $10^{-4}$ and $10^{-9}$, respectively. Values for $Nu$, $Re_{\text{LSC}}$ and $Re_{\text{centre}}$ at $Ha = 0$ can be found in the supplementary material of Zürner *et al.*, 2019, *J. Fluid Mech.* **876**, 1108–1128.

| $Ra$ | $Pr$ | $Pm$ | $Re_{\text{global}}$ | Figure |
|---|---|---|---|---|
| $(9.678 \pm 0.374) \times 10^5$ | 0.0292 | $1.362 \times 10^{-6}$ | $1545 \pm 144$ | |
| $(9.884 \pm 0.328) \times 10^5$ | 0.0292 | $1.362 \times 10^{-6}$ | $1485 \pm 135$ | |
| $(1.013 \pm 0.035) \times 10^6$ | 0.0292 | $1.362 \times 10^{-6}$ | $1560 \pm 146$ | |
| $(1.039 \pm 0.031) \times 10^6$ | 0.0292 | $1.362 \times 10^{-6}$ | $1664 \pm 151$ | |
| $(1.042 \pm 0.037) \times 10^6$ | 0.0292 | $1.362 \times 10^{-6}$ | $1463 \pm 154$ | |
| $(1.046 \pm 0.025) \times 10^6$ | 0.0292 | $1.362 \times 10^{-6}$ | $1602 \pm 142$ | |
| $(1.110 \pm 0.040) \times 10^6$ | 0.0292 | $1.362 \times 10^{-6}$ | $1735 \pm 168$ | |
| $(1.110 \pm 0.040) \times 10^6$ | 0.0292 | $1.362 \times 10^{-6}$ | $1612 \pm 163$ | |
| $(1.571 \pm 0.048) \times 10^6$ | 0.0292 | $1.362 \times 10^{-6}$ | $2003 \pm 173$ | |
| $(1.599 \pm 0.035) \times 10^6$ | 0.0292 | $1.362 \times 10^{-6}$ | $1977 \pm 184$ | |
| $(1.660 \pm 0.068) \times 10^6$ | 0.0292 | $1.362 \times 10^{-6}$ | $1762 \pm 215$ | |
| $(1.731 \pm 0.059) \times 10^6$ | 0.0292 | $1.362 \times 10^{-6}$ | $1963 \pm 203$ | |
| $(2.012 \pm 0.047) \times 10^6$ | 0.0292 | $1.362 \times 10^{-6}$ | $2213 \pm 217$ | |
| $(2.091 \pm 0.050) \times 10^6$ | 0.0292 | $1.362 \times 10^{-6}$ | $2367 \pm 238$ | |
| $(2.093 \pm 0.075) \times 10^6$ | 0.0292 | $1.362 \times 10^{-6}$ | $2193 \pm 229$ | |
| $(2.126 \pm 0.054) \times 10^6$ | 0.0292 | $1.362 \times 10^{-6}$ | $2151 \pm 196$ | |
| $(2.167 \pm 0.077) \times 10^6$ | 0.0292 | $1.362 \times 10^{-6}$ | $2172 \pm 217$ | 5(a) |
| $(2.177 \pm 0.052) \times 10^6$ | 0.0292 | $1.362 \times 10^{-6}$ | $2215 \pm 234$ | |
| $(2.270 \pm 0.053) \times 10^6$ | 0.0292 | $1.362 \times 10^{-6}$ | $2066 \pm 241$ | |
| $(2.301 \pm 0.059) \times 10^6$ | 0.0292 | $1.362 \times 10^{-6}$ | $2205 \pm 217$ | |
| $(3.120 \pm 0.071) \times 10^6$ | 0.0292 | $1.362 \times 10^{-6}$ | $2468 \pm 258$ | |
| $(3.125 \pm 0.078) \times 10^6$ | 0.0292 | $1.362 \times 10^{-6}$ | $2494 \pm 235$ | |
| $(3.139 \pm 0.070) \times 10^6$ | 0.0292 | $1.362 \times 10^{-6}$ | $2712 \pm 277$ | |
| $(3.192 \pm 0.087) \times 10^6$ | 0.0292 | $1.362 \times 10^{-6}$ | $2471 \pm 275$ | |
| $(4.101 \pm 0.081) \times 10^6$ | 0.0292 | $1.362 \times 10^{-6}$ | $2646 \pm 279$ | |
| $(4.143 \pm 0.167) \times 10^6$ | 0.0292 | $1.362 \times 10^{-6}$ | $3049 \pm 326$ | |

| | | | |
|---|---|---|---|
| $(4.179 \pm 0.132) \times 10^6$ | 0.0292 | $1.362 \times 10^{-6}$ | $2750 \pm 275$ |
| $(4.180 \pm 0.101) \times 10^6$ | 0.0292 | $1.362 \times 10^{-6}$ | $2941 \pm 308$ |
| $(4.182 \pm 0.145) \times 10^6$ | 0.0292 | $1.362 \times 10^{-6}$ | $2779 \pm 328$ |
| $(6.277 \pm 0.229) \times 10^6$ | 0.0292 | $1.362 \times 10^{-6}$ | $3340 \pm 382$ |
| $(6.340 \pm 0.157) \times 10^6$ | 0.0292 | $1.362 \times 10^{-6}$ | $3388 \pm 384$ |
| $(6.458 \pm 0.140) \times 10^6$ | 0.0292 | $1.362 \times 10^{-6}$ | $3178 \pm 355$ |
| $(6.496 \pm 0.189) \times 10^6$ | 0.0292 | $1.362 \times 10^{-6}$ | $3508 \pm 383$ |
| $(8.380 \pm 0.228) \times 10^6$ | 0.0292 | $1.362 \times 10^{-6}$ | $3770 \pm 504$ |
| $(8.681 \pm 0.290) \times 10^6$ | 0.0292 | $1.362 \times 10^{-6}$ | $3985 \pm 397$ |
| $(8.799 \pm 0.238) \times 10^6$ | 0.0292 | $1.362 \times 10^{-6}$ | $4223 \pm 397$ |
| $(9.854 \pm 0.281) \times 10^6$ | 0.0293 | $1.363 \times 10^{-6}$ | $4209 \pm 465$ |
| $(1.031 \pm 0.026) \times 10^7$ | 0.0292 | $1.362 \times 10^{-6}$ | $4315 \pm 439$ |
| $(1.043 \pm 0.022) \times 10^7$ | 0.0292 | $1.362 \times 10^{-6}$ | $3884 \pm 426$ |
| $(1.045 \pm 0.027) \times 10^7$ | 0.0292 | $1.362 \times 10^{-6}$ | $4107 \pm 487$ |
| $(1.045 \pm 0.030) \times 10^7$ | 0.0292 | $1.362 \times 10^{-6}$ | $4882 \pm 435$ |
| $(1.053 \pm 0.030) \times 10^7$ | 0.0292 | $1.362 \times 10^{-6}$ | $4233 \pm 486$ |
| $(1.254 \pm 0.030) \times 10^7$ | 0.0292 | $1.362 \times 10^{-6}$ | $4609 \pm 496$ |
| $(1.263 \pm 0.036) \times 10^7$ | 0.0292 | $1.362 \times 10^{-6}$ | $4728 \pm 467$ |
| $(1.270 \pm 0.033) \times 10^7$ | 0.0292 | $1.362 \times 10^{-6}$ | $4547 \pm 568$ |
| $(1.665 \pm 0.040) \times 10^7$ | 0.0292 | $1.362 \times 10^{-6}$ | $5328 \pm 582$ |
| $(1.672 \pm 0.044) \times 10^7$ | 0.0292 | $1.362 \times 10^{-6}$ | $5103 \pm 610$ |
| $(1.726 \pm 0.038) \times 10^7$ | 0.0292 | $1.361 \times 10^{-6}$ | $5109 \pm 631$ |
| $(1.805 \pm 0.042) \times 10^7$ | 0.0291 | $1.360 \times 10^{-6}$ | $4941 \pm 568$ |
| $(2.506 \pm 0.058) \times 10^7$ | 0.0292 | $1.361 \times 10^{-6}$ | $6087 \pm 733$ |
| $(2.531 \pm 0.061) \times 10^7$ | 0.0292 | $1.361 \times 10^{-6}$ | $5909 \pm 642$ |
| $(2.536 \pm 0.052) \times 10^7$ | 0.0292 | $1.361 \times 10^{-6}$ | $5903 \pm 680$ |
| $(2.547 \pm 0.055) \times 10^7$ | 0.0292 | $1.361 \times 10^{-6}$ | $6160 \pm 709$ |
| $(3.222 \pm 0.084) \times 10^7$ | 0.0292 | $1.362 \times 10^{-6}$ | $6501 \pm 780$ |
| $(3.318 \pm 0.088) \times 10^7$ | 0.0292 | $1.361 \times 10^{-6}$ | $7185 \pm 862$ |
| $(3.342 \pm 0.071) \times 10^7$ | 0.0292 | $1.361 \times 10^{-6}$ | $6653 \pm 776$ |
| $(3.344 \pm 0.065) \times 10^7$ | 0.0292 | $1.361 \times 10^{-6}$ | $6766 \pm 781$ |
| $(3.387 \pm 0.068) \times 10^7$ | 0.0292 | $1.360 \times 10^{-6}$ | $7162 \pm 874$ |
| $(4.824 \pm 0.100) \times 10^7$ | 0.0291 | $1.359 \times 10^{-6}$ | $7860 \pm 1006$ |
| $(4.853 \pm 0.095) \times 10^7$ | 0.0290 | $1.356 \times 10^{-6}$ | $8010 \pm 1008$ |
| $(5.113 \pm 0.098) \times 10^7$ | 0.0290 | $1.357 \times 10^{-6}$ | $8086 \pm 1029$ |
| $(5.281 \pm 0.098) \times 10^7$ | 0.0290 | $1.358 \times 10^{-6}$ | $8491 \pm 1091$ |
| $(5.813 \pm 0.112) \times 10^7$ | 0.0291 | $1.359 \times 10^{-6}$ | $8569 \pm 1058$ |
| $(5.816 \pm 0.118) \times 10^7$ | 0.0281 | $1.340 \times 10^{-6}$ | $8453 \pm 1106$ |
| $(5.894 \pm 0.127) \times 10^7$ | 0.0281 | $1.340 \times 10^{-6}$ | $8878 \pm 1171$ |
| $(5.934 \pm 0.130) \times 10^7$ | 0.0280 | $1.337 \times 10^{-6}$ | $8378 \pm 1138$ |

## Measurements with magnetic field

The uncertainties of $Pr$ and $Pm$ are, at most, $10^{-4}$ and $10^{-9}$, respectively.

| $Ra$ | $Ha$ | $Pr$ | $Pm$ | $Re_{\mathrm{global}}$ | $Nu$ | Regime | Figure |
|---|---|---|---|---|---|---|---|
| $(1.045 \pm 0.033) \times 10^6$ | $13.15 \pm 0.05$ | 0.0292 | $1.362 \times 10^{-6}$ | $1622 \pm 125$ | – | LSC: Oscillations | 2(a) |
| $(1.044 \pm 0.025) \times 10^6$ | $65.75 \pm 0.25$ | 0.0292 | $1.362 \times 10^{-6}$ | $1175 \pm 92$ | – | LSC: Oscillations | |
| $(1.043 \pm 0.036) \times 10^6$ | $65.75 \pm 0.25$ | 0.0292 | $1.362 \times 10^{-6}$ | $1153 \pm 81$ | – | LSC: Oscillations | |
| $(1.045 \pm 0.041) \times 10^6$ | $131.5 \pm 0.5$ | 0.0292 | $1.362 \times 10^{-6}$ | $617.7 \pm 33.8$ | – | LSC: No oscillations | |
| $(1.044 \pm 0.021) \times 10^6$ | $131.5 \pm 0.5$ | 0.0292 | $1.362 \times 10^{-6}$ | $695.6 \pm 46.8$ | – | LSC: No oscillations | 2(b) |
| $(1.044 \pm 0.020) \times 10^6$ | $263.0 \pm 1.0$ | 0.0292 | $1.362 \times 10^{-6}$ | $213.8 \pm 15.9$ | – | Cellular | |
| $(1.045 \pm 0.027) \times 10^6$ | $328.7 \pm 1.2$ | 0.0292 | $1.362 \times 10^{-6}$ | $198.9 \pm 54.3$ | – | Wall mode | |
| $(1.045 \pm 0.020) \times 10^6$ | $460.2 \pm 1.7$ | 0.0292 | $1.362 \times 10^{-6}$ | $176.3 \pm 61.0$ | – | Wall mode | |
| $(1.044 \pm 0.020) \times 10^6$ | $657.5 \pm 2.5$ | 0.0292 | $1.362 \times 10^{-6}$ | $144.0 \pm 12.5$ | – | Wall mode | |
| $(2.085 \pm 0.050) \times 10^6$ | $13.15 \pm 0.05$ | 0.0292 | $1.362 \times 10^{-6}$ | $2074 \pm 239$ | – | LSC: Oscillations | |
| $(2.090 \pm 0.052) \times 10^6$ | $13.15 \pm 0.05$ | 0.0292 | $1.362 \times 10^{-6}$ | $2030 \pm 219$ | – | LSC: Oscillations | |
| $(2.090 \pm 0.046) \times 10^6$ | $65.75 \pm 0.25$ | 0.0292 | $1.362 \times 10^{-6}$ | $1795 \pm 161$ | – | LSC: Oscillations | |
| $(2.089 \pm 0.040) \times 10^6$ | $65.75 \pm 0.25$ | 0.0292 | $1.362 \times 10^{-6}$ | $1696 \pm 149$ | – | LSC: Oscillations | |
| $(2.088 \pm 0.025) \times 10^6$ | $131.5 \pm 0.5$ | 0.0292 | $1.362 \times 10^{-6}$ | $1134 \pm 135$ | – | LSC: No oscillations | |
| $(2.089 \pm 0.023) \times 10^6$ | $131.5 \pm 0.5$ | 0.0292 | $1.362 \times 10^{-6}$ | $983.6 \pm 114.2$ | – | LSC: No oscillations | 5(a) |
| $(2.090 \pm 0.031) \times 10^6$ | $197.2 \pm 0.7$ | 0.0292 | $1.362 \times 10^{-6}$ | $535.9 \pm 21.8$ | – | LSC: No oscillations | |
| $(2.087 \pm 0.022) \times 10^6$ | $263.0 \pm 1.0$ | 0.0292 | $1.362 \times 10^{-6}$ | $449.4 \pm 56.4$ | – | LSC: No oscillations | |
| $(2.092 \pm 0.026) \times 10^6$ | $263.0 \pm 1.0$ | 0.0292 | $1.362 \times 10^{-6}$ | $398.3 \pm 32.1$ | – | Transition to cellular | |
| $(2.087 \pm 0.026) \times 10^6$ | $328.7 \pm 1.2$ | 0.0292 | $1.362 \times 10^{-6}$ | $434.5 \pm 96.0$ | – | Cellular | 5(a) |
| $(2.090 \pm 0.019) \times 10^6$ | $381.3 \pm 1.4$ | 0.0292 | $1.362 \times 10^{-6}$ | $347.4 \pm 73.3$ | – | Cellular | |
| $(2.090 \pm 0.021) \times 10^6$ | $427.4 \pm 1.6$ | 0.0292 | $1.362 \times 10^{-6}$ | $210.2 \pm 50.3$ | – | Wall mode | 5(a) |
| $(2.090 \pm 0.021) \times 10^6$ | $460.2 \pm 1.7$ | 0.0292 | $1.362 \times 10^{-6}$ | $277.8 \pm 129.8$ | – | Wall mode | 5(a) |
| $(2.089 \pm 0.022) \times 10^6$ | $657.5 \pm 2.5$ | 0.0292 | $1.362 \times 10^{-6}$ | $189.0 \pm 146.4$ | – | Wall mode | 5(a) |
| $(4.180 \pm 0.112) \times 10^6$ | $13.15 \pm 0.05$ | 0.0292 | $1.362 \times 10^{-6}$ | $2921 \pm 289$ | $7.59 \pm 0.80$ | LSC: Oscillations | |
| $(4.178 \pm 0.078) \times 10^6$ | $65.75 \pm 0.25$ | 0.0292 | $1.362 \times 10^{-6}$ | $2474 \pm 215$ | $7.49 \pm 0.48$ | LSC: Oscillations | |
| $(4.179 \pm 0.054) \times 10^6$ | $131.5 \pm 0.5$ | 0.0292 | $1.362 \times 10^{-6}$ | $1536 \pm 104$ | $5.99 \pm 0.39$ | LSC: Plume entrainment | |
| $(4.179 \pm 0.058) \times 10^6$ | $263.0 \pm 1.0$ | 0.0292 | $1.362 \times 10^{-6}$ | $788.8 \pm 114.4$ | – | Transition to cellular | |
| $(4.181 \pm 0.047) \times 10^6$ | $263.0 \pm 1.0$ | 0.0292 | $1.362 \times 10^{-6}$ | $680.7 \pm 124.3$ | – | Transition to cellular | |
| $(4.182 \pm 0.089) \times 10^6$ | $263.0 \pm 1.0$ | 0.0292 | $1.362 \times 10^{-6}$ | $700.1 \pm 80.7$ | – | Transition to cellular | |
| $(4.178 \pm 0.032) \times 10^6$ | $460.2 \pm 1.7$ | 0.0292 | $1.362 \times 10^{-6}$ | $522.4 \pm 52.3$ | – | Cellular | |
| $(4.178 \pm 0.023) \times 10^6$ | $591.7 \pm 2.2$ | 0.0292 | $1.362 \times 10^{-6}$ | $298.2 \pm 48.1$ | – | Cellular | 2(d), 3(a) |
| $(4.177 \pm 0.021) \times 10^6$ | $657.5 \pm 2.5$ | 0.0292 | $1.362 \times 10^{-6}$ | $134.4 \pm 14.8$ | – | Wall mode | |
| $(4.178 \pm 0.023) \times 10^6$ | $854.7 \pm 3.2$ | 0.0292 | $1.362 \times 10^{-6}$ | $122.4 \pm 25.1$ | – | Wall mode | |
| $(4.179 \pm 0.022) \times 10^6$ | $1052 \pm 4$ | 0.0292 | $1.362 \times 10^{-6}$ | $126.3 \pm 24.6$ | – | Wall mode | |

| | | | | | | | |
|---|---|---|---|---|---|---|---|
| $(6.268 \pm 0.164) \times 10^6$ | $13.15 \pm 0.05$ | 0.0292 | $1.362 \times 10^{-6}$ | $3306 \pm 346$ | $8.10 \pm 0.61$ | LSC: Oscillations | |
| $(6.271 \pm 0.123) \times 10^6$ | $65.75 \pm 0.25$ | 0.0292 | $1.362 \times 10^{-6}$ | $2743 \pm 279$ | $7.71 \pm 0.52$ | LSC: Oscillations | |
| $(6.271 \pm 0.075) \times 10^6$ | $131.5 \pm 0.5$ | 0.0292 | $1.362 \times 10^{-6}$ | $1919 \pm 152$ | $7.28 \pm 0.39$ | LSC: Plume entrainment | |
| $(6.263 \pm 0.067) \times 10^6$ | $263.0 \pm 1.0$ | 0.0292 | $1.362 \times 10^{-6}$ | $1068 \pm 166$ | $5.48 \pm 0.40$ | Transition to cellular | |
| $(6.268 \pm 0.025) \times 10^6$ | $460.2 \pm 1.7$ | 0.0292 | $1.362 \times 10^{-6}$ | $424.8 \pm 100.9$ | – | Cellular | |
| $(6.270 \pm 0.022) \times 10^6$ | $657.5 \pm 2.5$ | 0.0292 | $1.362 \times 10^{-6}$ | $328.6 \pm 81.9$ | – | Cellular | |
| $(6.269 \pm 0.031) \times 10^6$ | $854.7 \pm 3.2$ | 0.0292 | $1.362 \times 10^{-6}$ | $99.47 \pm 12.31$ | – | Wall mode | |
| $(6.268 \pm 0.022) \times 10^6$ | $1052 \pm 4$ | 0.0292 | $1.362 \times 10^{-6}$ | $87.35 \pm 18.06$ | – | Wall mode | |
| $(1.045 \pm 0.027) \times 10^7$ | $13.15 \pm 0.05$ | 0.0292 | $1.362 \times 10^{-6}$ | $4221 \pm 431$ | $9.19 \pm 0.71$ | LSC: Oscillations | |
| $(1.045 \pm 0.028) \times 10^7$ | $65.76 \pm 0.25$ | 0.0292 | $1.362 \times 10^{-6}$ | $3486 \pm 364$ | $9.23 \pm 0.80$ | LSC: Oscillations | 4(b) |
| $(1.045 \pm 0.018) \times 10^7$ | $65.76 \pm 0.25$ | 0.0292 | $1.362 \times 10^{-6}$ | $3607 \pm 404$ | – | LSC: Oscillations | |
| $(1.045 \pm 0.012) \times 10^7$ | $131.5 \pm 0.5$ | 0.0292 | $1.362 \times 10^{-6}$ | $2451 \pm 231$ | $9.07 \pm 0.35$ | LSC: Plume entrainment | |
| $(1.045 \pm 0.013) \times 10^7$ | $131.5 \pm 0.5$ | 0.0292 | $1.362 \times 10^{-6}$ | $2579 \pm 306$ | – | LSC: Plume entrainment | |
| $(1.045 \pm 0.009) \times 10^7$ | $197.3 \pm 0.7$ | 0.0292 | $1.362 \times 10^{-6}$ | $1746 \pm 110$ | $7.67 \pm 0.28$ | LSC: Plume entrainment | |
| $(1.045 \pm 0.017) \times 10^7$ | $263.0 \pm 1.0$ | 0.0292 | $1.362 \times 10^{-6}$ | $1320 \pm 235$ | – | LSC: Plume entrainment | |
| $(1.045 \pm 0.015) \times 10^7$ | $263.0 \pm 1.0$ | 0.0292 | $1.362 \times 10^{-6}$ | $1049 \pm 151$ | $6.62 \pm 0.40$ | LSC: Plume entrainment | |
| $(1.044 \pm 0.007) \times 10^7$ | $460.3 \pm 1.7$ | 0.0292 | $1.362 \times 10^{-6}$ | $745.9 \pm 221.4$ | $5.05 \pm 0.31$ | Cellular | 4(c) |
| $(1.045 \pm 0.010) \times 10^7$ | $460.3 \pm 1.7$ | 0.0292 | $1.362 \times 10^{-6}$ | $763.0 \pm 201.5$ | – | Cellular | |
| $(1.045 \pm 0.003) \times 10^7$ | $657.5 \pm 2.5$ | 0.0292 | $1.362 \times 10^{-6}$ | – | $3.18 \pm 0.14$ | Cellular | |
| $(1.044 \pm 0.003) \times 10^7$ | $657.5 \pm 2.5$ | 0.0292 | $1.362 \times 10^{-6}$ | $661.7 \pm 91.1$ | $3.67 \pm 0.17$ | Cellular | |
| $(1.045 \pm 0.004) \times 10^7$ | $657.5 \pm 2.5$ | 0.0292 | $1.362 \times 10^{-6}$ | $430.4 \pm 54.2$ | $3.18 \pm 0.15$ | Cellular | |
| $(1.045 \pm 0.002) \times 10^7$ | $657.5 \pm 2.5$ | 0.0292 | $1.362 \times 10^{-6}$ | $579.8 \pm 144.6$ | – | Cellular | |
| $(1.045 \pm 0.007) \times 10^7$ | $657.5 \pm 2.5$ | 0.0292 | $1.362 \times 10^{-6}$ | $698.4 \pm 124.6$ | $3.41 \pm 0.20$ | Cellular | |
| $(1.045 \pm 0.002) \times 10^7$ | $854.8 \pm 3.2$ | 0.0292 | $1.362 \times 10^{-6}$ | $409.2 \pm 61.8$ | – | Cellular | 4(d) |
| $(1.044 \pm 0.002) \times 10^7$ | $1052 \pm 4$ | 0.0292 | $1.362 \times 10^{-6}$ | $116.7 \pm 33.1$ | – | Wall mode | 2(e), 4(e) |
| $(1.671 \pm 0.043) \times 10^7$ | $13.15 \pm 0.05$ | 0.0292 | $1.362 \times 10^{-6}$ | $5240 \pm 590$ | $11.0 \pm 0.8$ | LSC: Oscillations | |
| $(1.670 \pm 0.034) \times 10^7$ | $65.77 \pm 0.25$ | 0.0292 | $1.362 \times 10^{-6}$ | $4670 \pm 495$ | $10.9 \pm 0.6$ | LSC: Oscillations | |
| $(1.671 \pm 0.021) \times 10^7$ | $131.5 \pm 0.5$ | 0.0292 | $1.362 \times 10^{-6}$ | $3633 \pm 302$ | $10.9 \pm 0.4$ | LSC: Plume entrainment | |
| $(1.672 \pm 0.021) \times 10^7$ | $263.1 \pm 1.0$ | 0.0292 | $1.362 \times 10^{-6}$ | $1695 \pm 206$ | $8.55 \pm 0.36$ | LSC: Plume entrainment | |
| $(1.672 \pm 0.015) \times 10^7$ | $460.3 \pm 1.7$ | 0.0292 | $1.362 \times 10^{-6}$ | $1180 \pm 179$ | $6.75 \pm 0.27$ | Cellular | |
| $(1.670 \pm 0.013) \times 10^7$ | $657.6 \pm 2.5$ | 0.0292 | $1.362 \times 10^{-6}$ | $690.5 \pm 229.8$ | $4.98 \pm 0.26$ | Cellular | |
| $(1.671 \pm 0.002) \times 10^7$ | $854.8 \pm 3.2$ | 0.0292 | $1.362 \times 10^{-6}$ | $904.8 \pm 176.5$ | $3.63 \pm 0.13$ | Cellular | |
| $(1.671 \pm 0.003) \times 10^7$ | $1052 \pm 4$ | 0.0292 | $1.362 \times 10^{-6}$ | $408.7 \pm 97.6$ | $2.97 \pm 0.12$ | Cellular | |
| $(2.508 \pm 0.063) \times 10^7$ | $65.79 \pm 0.25$ | 0.0292 | $1.361 \times 10^{-6}$ | $5385 \pm 634$ | $11.6 \pm 0.7$ | LSC: Oscillations | |
| $(2.510 \pm 0.033) \times 10^7$ | $131.6 \pm 0.5$ | 0.0292 | $1.361 \times 10^{-6}$ | $4545 \pm 458$ | $11.8 \pm 0.3$ | LSC: Plume entrainment | |
| $(2.507 \pm 0.030) \times 10^7$ | $263.1 \pm 1.0$ | 0.0292 | $1.362 \times 10^{-6}$ | $2514 \pm 497$ | $9.77 \pm 0.33$ | LSC: Plume entrainment | |
| $(3.342 \pm 0.073) \times 10^7$ | $13.16 \pm 0.05$ | 0.0292 | $1.361 \times 10^{-6}$ | $7043 \pm 832$ | $12.5 \pm 0.6$ | LSC: Oscillations | |
| $(3.337 \pm 0.073) \times 10^7$ | $65.81 \pm 0.25$ | 0.0292 | $1.361 \times 10^{-6}$ | $6164 \pm 805$ | $12.3 \pm 0.6$ | LSC: Oscillations | |

| | | | | | | | |
|---|---|---|---|---|---|---|---|
| $(3.343 \pm 0.041) \times 10^7$ | $131.6 \pm 0.5$ | 0.0292 | $1.361 \times 10^{-6}$ | $6361 \pm 587$ | $12.3 \pm 0.4$ | LSC: Plume entrainment | |
| $(3.344 \pm 0.035) \times 10^7$ | $263.2 \pm 1.0$ | 0.0292 | $1.361 \times 10^{-6}$ | $2675 \pm 357$ | $11.0 \pm 0.3$ | LSC: Plume entrainment | |
| $(3.345 \pm 0.035) \times 10^7$ | $263.2 \pm 1.0$ | 0.0292 | $1.361 \times 10^{-6}$ | $2542 \pm 323$ | $10.8 \pm 0.3$ | LSC: Plume entrainment | |
| $(3.340 \pm 0.048) \times 10^7$ | $460.5 \pm 1.7$ | 0.0292 | $1.361 \times 10^{-6}$ | $1658 \pm 392$ | $8.84 \pm 0.41$ | Transition to cellular | |
| $(3.344 \pm 0.039) \times 10^7$ | $657.8 \pm 2.5$ | 0.0292 | $1.362 \times 10^{-6}$ | $1311 \pm 396$ | $7.20 \pm 0.30$ | Cellular | |
| $(3.345 \pm 0.030) \times 10^7$ | $855.1 \pm 3.2$ | 0.0292 | $1.362 \times 10^{-6}$ | $1207 \pm 467$ | $5.90 \pm 0.25$ | Cellular | |
| $(3.342 \pm 0.008) \times 10^7$ | $1052 \pm 4$ | 0.0292 | $1.362 \times 10^{-6}$ | $854.2 \pm 246.8$ | $4.75 \pm 0.19$ | Cellular | |
| $(3.344 \pm 0.006) \times 10^7$ | $1052 \pm 4$ | 0.0292 | $1.362 \times 10^{-6}$ | $1261 \pm 375$ | $5.12 \pm 0.16$ | Cellular | |
| $(3.346 \pm 0.009) \times 10^7$ | $1052 \pm 4$ | 0.0292 | $1.362 \times 10^{-6}$ | $878.8 \pm 298.2$ | $4.88 \pm 0.15$ | Cellular | |
| $(5.822 \pm 0.114) \times 10^7$ | $13.18 \pm 0.05$ | 0.0291 | $1.359 \times 10^{-6}$ | $8329 \pm 1024$ | $15.7 \pm 0.9$ | LSC: Oscillations | |
| $(5.914 \pm 0.141) \times 10^7$ | $13.35 \pm 0.06$ | 0.0282 | $1.341 \times 10^{-6}$ | $8542 \pm 1069$ | $15.7 \pm 0.9$ | LSC: Oscillations | |
| $(5.807 \pm 0.115) \times 10^7$ | $65.89 \pm 0.25$ | 0.0291 | $1.359 \times 10^{-6}$ | $7589 \pm 1070$ | $15.2 \pm 0.9$ | LSC: Oscillations | |
| $(5.840 \pm 0.084) \times 10^7$ | $131.8 \pm 0.5$ | 0.0291 | $1.359 \times 10^{-6}$ | $6453 \pm 758$ | $15.0 \pm 0.7$ | LSC: Oscillations | |
| $(5.820 \pm 0.074) \times 10^7$ | $131.8 \pm 0.5$ | 0.0291 | $1.359 \times 10^{-6}$ | $6638 \pm 648$ | $15.5 \pm 0.5$ | LSC: Oscillations | |
| $(5.777 \pm 0.086) \times 10^7$ | $131.8 \pm 0.5$ | 0.0291 | $1.359 \times 10^{-6}$ | $6328 \pm 734$ | $15.5 \pm 0.6$ | LSC: Oscillations | |
| $(5.855 \pm 0.056) \times 10^7$ | $263.4 \pm 1.0$ | 0.0291 | $1.360 \times 10^{-6}$ | $3926 \pm 385$ | $14.3 \pm 0.4$ | LSC: Plume entrainment | 2(c) |
| $(5.852 \pm 0.063) \times 10^7$ | $263.5 \pm 1.0$ | 0.0291 | $1.360 \times 10^{-6}$ | $3861 \pm 488$ | $14.0 \pm 0.5$ | LSC: Plume entrainment | |
| $(5.845 \pm 0.057) \times 10^7$ | $263.5 \pm 1.0$ | 0.0291 | $1.360 \times 10^{-6}$ | $3844 \pm 415$ | $14.4 \pm 0.4$ | LSC: Plume entrainment | |
| $(5.839 \pm 0.054) \times 10^7$ | $263.5 \pm 1.0$ | 0.0291 | $1.360 \times 10^{-6}$ | $3857 \pm 398$ | $14.4 \pm 0.4$ | LSC: Plume entrainment | |
| $(5.849 \pm 0.100) \times 10^7$ | $460.9 \pm 1.8$ | 0.0291 | $1.360 \times 10^{-6}$ | $2576 \pm 590$ | $12.0 \pm 0.6$ | Transition to cellular | |
| $(5.855 \pm 0.051) \times 10^7$ | $658.3 \pm 2.5$ | 0.0292 | $1.361 \times 10^{-6}$ | $2257 \pm 648$ | $10.1 \pm 0.3$ | Cellular | |
| $(5.855 \pm 0.039) \times 10^7$ | $855.6 \pm 3.2$ | 0.0292 | $1.361 \times 10^{-6}$ | $1531 \pm 486$ | $8.89 \pm 0.31$ | Cellular | |
| $(5.853 \pm 0.023) \times 10^7$ | $1053 \pm 4$ | 0.0292 | $1.361 \times 10^{-6}$ | $1436 \pm 557$ | $7.63 \pm 0.27$ | Cellular | |
